# Supplementary material for: A Lightweight CNN Model for Detecting Respiratory Diseases from Lung Auscultation Sounds using EMD-CWT-based Hybrid Scalogram
Source: arXiv:2009.04402 source file (2020-09-08)
Supplement: Supplementary file 1 [file appendix.tex]

\clearpage
\refstepcounter{dummy}
\pdfbookmark[0]{Appendix}{appendix}

\begingroup
\hypersetup{bookmarksopenlevel=2}

\subfoilhead[-\baselineskip]{%
  \texorpdfstring{Reusing of informations}{\cms{maketitle}}%
}
\noindent
Using of data that are available in \code[red]<\maketitle>.%
\Remark{This example is first published by Sebastian Rahtz in the
  mailing list `pdftex'.
}\\
\Green{Caution}: This only works before the first page is shipped out.
\begin{verbatim}
\newcommand{\org@maketitle}{}$commentchar$textsl( $textsf($LaTeX-Check))
\let\org@maketitle\maketitle
\def\maketitle{$commentchar
  \hypersetup{
    $Blue(pdftitle)={$Red(\@title)},
    $Blue(pdfauthor)={$Red(\@author)}
  }$commentchar
  \org@maketitle
}
\end{verbatim}

\subfoilhead{Tasks of encoding command \cms{OT1}\cms{ss}}
\begin{itemize}
\item In a protected environment it expands to \cms{noexpand} \cms{ss}.
\item Warning, if used in math mode.
\item The character (\cms{OT1}\cms{ss} = \cms{char}\Code{\string"19}) is set, 
      if the currently active encoding matches.
\item Else the value of the default encoding (\cms{?}\cms{ss}) is used\\
      (\cms{?}\cms{ss} = \cms{UseTextSymbol}\Code{\{OT1\}}\cms{ss}).
\end{itemize}

\subfoilhead[-\baselineskip]{Bookmarks by \cms{addcontentsline}}
\label{sec:addcontentsline}

\begin{itemize}
\item \Red{\cms{addcontentsline}} also adds a bookmark entry:
      \begin{quote}\small
        \cms{section\string*}\Code{\{Starred section\}}\\
        \Red{\cms{addcontentsline}}\Code{\{toc\}\{section\}%
          \{Starred section\}}
      \end{quote}
\item For the link the \empty{last valid target (destination)} is used.
\item If there is a warning ``\Green{contentsline with no destination}'',
      a dummy target can be created:
      \begin{quote}\small
        \Blue{\cms{newcounter}\Code{\{dummy\}}}\\
        \cms{begin}\Code{\{document\}}\\
        *ind*\Blue{\cms{refstepcounter}\Code{\{dummy\}}}\\
        *ind*\Red{\cms{addcontentsline}}\Code{\{toc\}\{section\}%
          \{Contents\}}
      \end{quote}
\end{itemize}

\subfoilhead[-\baselineskip]{Definition of \cms{texorpdfstring}}

\begin{itemize}
\item \cms{pdfstringdef} sets a switch \Blue{\cms{ifHy@pdfstring}}.
\item \cms{texorpdfstring} is full expandable:
\newcommand\thisremark{%
  \Remark[\\@firstoftwo, \\@secondoftwo]{%
    Commands of the \LaTeX-Kernel:\r
    \r
    \space\space\\long \\def \\@firstoftwo \string\t\#1\#2\{\#1\}\r
    \space\space\\long \\def \\@secondoftwo \string\t\#1\#2\{\#2\}\r
    \r
    is the same as:\r
    \r
    \space\space\\newcommand\{\\@firstoftwo\}[2]\{\#1\}\r
    \space\space\\newcommand\{\\@secondoftwo\}[2]\{\#2\}%
  }%
}
\begin{verbatim}
\newcommand$string*{$Red(\texorpdfstring){$commentchar
  $Blue(\ifHy@pdfstring)
    \expandafter\@secondoftwo$thisremark
  $Blue(\else)
    \expandafter\@firstoftwo
  $Blue(\fi)
}
\end{verbatim}
\end{itemize}

\subsubfoilhead[-\baselineskip]{Examples for \cms{texorpdfstring}}

Syntax: \Red{\cms{texorpdfstring}}\Code{\Green{\{\textsl{*tex* string}\}}%
  \Blue{\{\textsl{*pdf* string}\}}}

\begin{quote}
  \cms{section}\Code{\{Pythagoras:}\\
  *ind*\Red{\cms{texorpdfstring}}%
    \Code{\Green{\{\$ a\string^2 + b\string^2 = c\string^2 \$\}}%
      \Blue{\{}\commentchar}\\
  *ind**ind*\Blue{\Code{a}\cms{texttwosuperior}\cms{ }\Code{+ b}%
    \cms{texttwosuperior}\cms{ }\Code{=}}\\
  *ind**ind*\Blue{\Code{c}\cms{texttwosuperior}\Code{\}}}\commentchar\\
  \Code{\}}\\
  \cms{section}\Code{\{\commentchar}\\
  *ind*\Red{\cms{texorpdfstring}}%
    \Green{\Code{\{}\cms{textcolor}\Code{\{red\}\}}}\Code{\Blue{\{\}}%
    \{Red\} Mars\commentchar}\\
  \Code{\}}
\end{quote}

\subfoilhead{Properties of \abbr{hypbmsec}}

\begin{itemize}
\item Should work with packages that do not change the syntax
      of the\\
      \cms{section} commands. *hypbmsec* should be
      loaded \Blue{last}.
\item Works \Blue{without} *hyperref* (bookmark argument is ignored).
\item \Blue{Parameter delimiters} \Green{inside} the
      optional parameter are protected\\
      by \Red{curly braces}:
\begin{quote}
  \Code{(\dots\Blue(\dots\Red\{\Blue)\Red\}\dots)}%
  \quad or\quad
  \Code{[\Red\{\dots\Blue[\dots\Blue]\dots\Red\}]}
\end{quote}
\end{itemize}

\subfoilhead[-\baselineskip]{\texorpdfstring
  {General document information}%
  {/CreationDate and /ModDate}%
}

\begin{Nav}{\NavInfo}

\noindent
Example for setting
\Blue{\Code{/CreationDate}} and \Blue{\Code{/ModDate}}:

\begin{smallpar}
  \noindent
  \Red{\cms{pdfinfo}}\Code{\{\Blue{/CreationDate} (D:19990909000000-01'00')\}}\\
  \cms{begingroup}\\
  *ind*\cms{def}\cms{twodigits}\Code{\#1\{}%
    \cms{ifnum}\Code{\#1<10 0}\cms{fi}\cms{the}\Code{\#1\}\commentchar}\\
  *ind*\cms{count}\Code{0=}\cms{time}\Code{ }%
    \cms{divide}\cms{count}\Code{0 by 60}\\
  *ind*\cms{edef}\cms{x}\Code{\{}%
    \cms{twodigits}\Code{\{}\cms{count}\Code{0\}\}\commentchar}\\
  *ind*\cms{multiply}\cms{count}\Code{0 by 60}\\
  *ind*\cms{count}\Code{1=}\cms{time}\Code{ }%
    \cms{advance}\cms{count}\Code{1 by -}\cms{count}\Code{0}\\
  *ind*\cms{edef}\cms{x}\Code{\{}%
    \cms{x}\cms{twodigits}\Code{\{}\cms{count}\Code{1\}\}\commentchar}\\
  *ind*\cms{edef}\cms{x}\Code{\{\Blue{/ModDate} (D:}\cms{the}\cms{year}\\
  *ind**ind*\cms{twodigits}\cms{month}\Code{ }%
    \cms{twodigits}\cms{day}\Code{ }\cms{x}\Code{ 00-01'00')\}\commentchar}\\
  \cms{expandafter}\cms{endgroup}\\
  \cms{expandafter}\Red{\cms{pdfinfo}}\cms{expandafter}%
    \Code{\{}\cms{x}\Code{\}\commentchar}
\end{smallpar}

\end{Nav}

\subfoilhead[-1.5\baselineskip]{\texorpdfstring{Example for }{}%
  \abbr{``}Named Actions\abbr{''}%
%  `Named Actions'%
}

  \begin{smallpar}
\begin{verbatim}
\newcommand{\bmaction}[3][$Blue(0)]{$textsl%
  \begingroup
    $Red(\pdfstringdef)\x{#3}$textsl%
    $Red(\pdfoutline)
      $empty(user {)<< /S /Named /N /$Blue(#2) >>$empty(}) 
        $empty(count) $Blue(#1) $empty({)\x$empty(})$textsl%
  \endgroup
}
\bmaction[$Blue(-3)]{$Green(NOP)}{Navigation}
  \bmaction[$Blue(2)]{$Green(FullScreen)}{Full-screen}
    \bmaction{$Green(PageOnly)}{Page only}
    \bmaction{$Green(ShowThumbs)}{Thumbnails}
  \bmaction[$Blue(6)]{$Green(NOP)}{Selecting pages}
    \bmaction{$Green(PrevPage)}{Previous page}
    $dots
\end{verbatim}
  \end{smallpar}

\SetNav{\NavFull\NavSep\NavPrev\NavSep\NavQuit}
\endgroup
\endinput
